# Supplementary material for: Study of charmonium production via the decay to $p\bar{p}$ at $\sqrt{s} = 13 TeV$
Source: arXiv:2407.14261 source file (2025-01-28)
Supplement: Supplementary file 1 [file supplementary-app.tex]

\clearpage

\section{Supplementary material for LHCb-PAPER-2024-004}
\label{sec:Supplementary-App}

% This appendix contains supplementary material that will be posted
% on the public CDS record but will not appear in the paper.

% Please leave the above sentence in your draft for first and 
% second circulation and replace what follows by your actual supplementary material.
% For more information about other types of supplementary material, see Section~\ref{sec:Supplementary}. Plots and tables that follow should be well described, either with captions or with additional explanatory text.

% \begin{figure}[!htb]
%   \begin{center}
%     \includegraphics[scale=0.65,bb=50 300 580 700,clip=true]{Roger-plot}
%     \vspace*{-1.0cm}
%   \end{center}
%   \caption{
%     \small %captions should be a little bit smaller than main text
%     Comparison of our result to those from other experiments.
%     Note that the style of this figure differs slightly from that of Figure~\ref{fig:example}}
%   \label{fig:roger}
% \end{figure}

\clearpage
