# Supplementary material for: Study of charmonium production via the decay to $p\bar{p}$ at $\sqrt{s} = 13 TeV$
Source: arXiv:2407.14261 source file (2025-01-28)
Supplement: Supplementary file 2 [file supplementary.tex]

\section{Inclusion of supplementary material}
\label{sec:Supplementary}
